# Supplementary material for: Recycling Scraps: Improving Private Learning by Leveraging Intermediate Checkpoints
Source: arXiv:2210.01864 source file (2024-09-17)
Supplement: Supplementary file 1 [file misc_appendix.tex]

\section{Related work}

\mypar{Privacy-preserving ML} ML models are well known to unintentionally memorize private information about their training data. This has led to a long line of research that demonstrates various attacks that extract private information from ML models, e.g., membership inference~\cite{shokri2017membership,mahloujifar2022property,carlini2022membership,shejwalkar2021membership}, attribute inference~\cite{melis2019exploiting}, text extraction~\cite{carlini2021extracting,carlini2019secret}, model inversion~\cite{fredrikson2014privacy,fredrikson2015model}, etc. To mitigate such private information leakage, various privacy preserving ML algorithms are proposed~\cite{shejwalkar2021privacy,tang2022mitigating,nasr2018machine,DP-DL,thakkar2019differentially} that aim to reduce memorization during training. 

\mypar{Differentially private ML}
Differential privacy (DP) is the gold standard of privacy, and hence, the differential privacy based defenses~\citep{chaudhuri2011differentially,DP-DL,thakkar2019differentially} that add carefully calibrated noise to provide rigorous DP guarantees are widely adopted. In fact, differentially private stochastic gradient decent (DP-SGD)~\cite{song2013stochastic,BST14,DP-DL} has become the state-of-the-art in training private deep learning models~\cite{mcmahan2018general,mcmahan2018learning,esa++,papernot2020tempered,ramaswamy2020training,andrew2021differentially}. Unfortunately, due to the noise addition during training, DP-SGD often leads to undesired trade-offs between privacy and utility of its resulting models, and improving these trade-offs is an important and active area of research. The literature has proposed various methods to improve the DP-SGD trade-offs~\cite{balle2020privacy,tramer2020differentially,amid2022public,de2022unlocking,kairouz2021practical}.

\mypar{Checkpoints aggregations}
The idea of aggregating intermediate training checkpoints to improve performance has been previously explored, but mainly in non-private settings~\cite{chen2017checkpoint,izmailov2018averaging}. 
Furthermore, performance gains due to checkpoints aggregations are negligible in non-private settings, probably due to the state-of-the-art performances of ML algorithms such as SGD and Adam in non-private settings.
Recently De et al.~\cite{de2022unlocking} demonstrated that exponential moving average (EMA) aggregation can help improve performance of DP-SGD trained ML models. However, we propose better aggregation algorithms that outperform EMA as well as show that the choice of EMA coefficient in~\cite{de2022unlocking} is sub-optimal and can be easily improved.

\mypar{Uncertainty quantification in ML}
As discussed in Section~\ref{intro}, uncertainty quantification (UQ) is instrumental for reliability of ML based systems, and hence, the field of UQ in non-private ML has a long history of research~\cite{mitchell1980need,kabir2018neural,roy2018inherent,hubschneider2019calibrating,tagasovska2019single,begoli2019need,mcdermott2019deep,wang2019aleatoric,nair2020exploring,abdar2021review}. 
All of these works deal with non-private ML and, to the best of our knowledge, there is no work that studies UQ in DP setting. For brevity, we do not elaborate more on the prior works on UQ in non-private ML, and refer the interested readers to comprehensive reviews in~\cite{kabir2018neural,abdar2021review}.
